# Supplementary material for: LSST Science Book, Version 2.0
Source: arXiv:0912.0201 source file (2009-12-01)
Supplement: Supplementary file 1 [file imsim.tex]

% ======================================================================
%+
% NAME:
%   appendix/imagesim/imsim.tex
%
% PURPOSE:
%
%
% COMMENTS:
%
%
%
%
%    
% INPUTS:
%
%
%
% OPTIONAL INPUTS:
%
%
% OUTPUTS:
%
%
% DEPENDENCIES:
%
%
%
%
% EXAMPLES:
%
%
%   
% BUGS:
%
%
% AUTHORS:
%  JRP
%
%-
% ======================================================================
\section[Image Simulations]{Image Simulations}
\label{sec:design:imsim}

{\it John Peterson, Garrett Jernigan,
  Andrew Connolly, Justin Bankert, Rob Gibson, Kirk Gilmore, Emily Grace, R. Lynne Jones, Steve
  Kahn, Alan Meert, Suzanne Nichols, James
  Pizagno, Andrew Rasmussen, Simon Krughoff}

High-fidelity image simulations are required to test how well the
instrument design and data analysis pipelines will achieve the LSST
science goals.  To that end, an Image Simulation Team has formed to
provide high fidelity end-to-end simulations of the sky. These
simulated images and catalogs extend to $r = 28$ (deeper than the expected
ten year depth of the LSST coadded images) and are used in designing
and testing algorithms for the use by the data management groups,
evaluating the capabilities and scalability of the reduction and
analysis pipelines, testing and optimizing the scientific returns of
the LSST survey and providing realistic LSST data to the science
collaborations to evaluate the expected performance of LSST.
\autoref{fig:flow} shows the flow of data through the LSST
simulation framework. 

\begin{figure}[ht!]
  \centerline{\resizebox{!}{5in}{\includegraphics{appendix/imagesim/FlowChart.png}}}
  \caption{The flow of information through the image simulation. The
    top level describes a static view of the sky that is sampled to
    provide instance catalogs (based on the operations simulations, \autoref{sec:design:opsim}). These
    catalogs are then passed into the image simulator resulting in a
    set of FITS images and catalogs. \label{fig:flow}}
\end{figure}

The image simulator \citep{peterson05} %is a set of fast codes that
follows photons from a catalog of objects (that are possibly lensed)
through the atmosphere, refracted and reflected through the optics,
and recorded in a detector simulator. The simulation is high fidelity
in that all wavelength-dependent optics, detector, and atmospheric
effects are included. The simulator is also fast enough for us to be
able to simulate 3 Gigapixel images, like those that will be obtained
with LSST, in $\sim $6 or 7 hours using a large pool of parallel
machines. 

First, the simulator starts from a catalog of objects. Catalogs from
cosmological and Galactic structure models ({\em base catalogs}) are
stored with a database enabling the generation of a view of the sky
above the atmosphere. These base catalogs
%are derived from different simulation groups and 
include the
spectral, photometric, astrometric and morphological properties of the
astronomical sources. 
%This static view of the sky is being extended to
%include transient events and moving sources (e.g. supernovae, variable
%stars and AGN, proper motions and Solar System objects).
The base catalogs are queried based on simulated observation sequences
from the operational simulator (\autoref{sec:design:opsim}) creating a
series of {\em instance catalogs}. 
%At this point, the catalogs are output, with
%associated uncertainties, as LSST simulated catalogs and are
%reformatted for input into the image simulator.
Given the time, RA and Dec of each
pointing, the appropriate airmass, sky background and observing
conditions can be determined (as well as incorporating variability and
moving sources). 

Each object in the catalog has a sky position, magnitude at some
wavelength, and spectral energy distribution file to determine the
wavelengths of photons. Each object can either be represented by a set
of parameters describing a spatial model or a hyper-resolved image to
determine the probability distribution of where the photons are
emitted. Additionally, objects could vary in flux during the exposure,
they could move during the exposure (in the case of Solar System
objects), or they could have shear distortion parameters to distort
the locations of the photons due to gravitational lensing. Photons are
drawn from this catalog in proportion to their magnitude and both the
SED and spatial model are sampled. In this way, photons are chosen one
at a time with two sky positions, a wavelength, and a time.

The Millennium Simulation galaxy catalog \citep{K+W07} includes 
proper baryon physics (including feedback and dust) into the pure dark matter Millennium Simulation,
and should reproduce the color, luminosity, and clustering distribution observed
in large and deep surveys. We therefore use this as our galaxy
catalog. 
%The baryonic physics in the
%\cite{K+W07} models include gas cooling, heating from star
%formation, supernovae, and 'radio mode' feedback. A model for the ISM
%dust produces an excellent match between color-luminosity relation
%seen in deep surveys. The size of the Millennium Simulation in
%luminosity and redshift allows the Image Simulation software to
%reproduce the of depth and area goals targeted by LSST. The models of
The Millennium Simulation follows galaxies in a 
%box that is 500 Mpc h$^{-1}$, on a side, simulating a 
light-cone survey with an area of
11.5$\times$2.3-deg$^2$ out to a redshift of $z = 1$ and that has no repeating
objects. This then is tiled across the sky to get the LSST sky
coverage. 

%To meet LSST photometric science goals, a detailed modeling of the SED
%for all objects in the Image Simulator is required. Including detailed
%baryonic physics allows 
The SED of each galaxy is estimated using
the \cite{bruzual03} stellar population models. The
\cite{K+W07} models provide SDSS {\it g, r, i, z}-band
magnitudes, Johnson Filter K-band magnitudes, and redshift for every
galaxy, which allows for the \cite{bruzual03} model spectra to be fit
to the galaxies. With the appropriate full SED and redshift, the LSST
apparent magnitudes can be calculated. 
%This allows a characterization
%of each simulated galaxies star formation history. 
Every galaxy is assigned a realistic morphological
profile, including a disk-to-total flux
ratio, position angle in the sky, inclination along the line-of-sight,
bulge radius, and disk radius. 
More accurate galaxy profiles,
including high-frequency spatial structure such as HII regions and
spiral arms, can be simulated using FITS images as input into the
Image Simulator. 
%The use of more detailed galaxy morphological
%profiles in the Image Simulator will allow LSST to study how galaxy
%morphology varies with environment and redshift.

Currently, stars are included in the Image Simulator with full SED
(from \citealt{Kurucz79} models),
spatial velocities, and positions.  
%Selecting stellar populations with
%a wide range in spatial distribution and velocity parameters will
%demonstrate LSST's science-goal of mapping the Milky Way's
%structure. The SEDs for stars are derived from Kurucz models. 
The model used to generate main sequence stars is based on a model from 
\citet{juric08}, as detailed in \autoref{Sec:stellarCounts}.
The model includes user-specified amounts of
thick-disk, thin-disk, and halo stars. Each version of a catalog
contains metadata on metallicity, temperature, luminosity-type, and
surface gravity, allowing the user to search for correlations between
observed LSST photometry and physical information about stars using
the simulated data. The catalog will be updated to include dwarf and
giant stars.

After the photons are selected from the astronomical source list, the
photons begin at the top of the atmosphere in a simulation of
atmospheric turbulence.  Our model of the atmosphere is constructed by
generating atmospheric screens.
%$ like those in
%$\autoref{fig:imsim5}. 
These screens model the density fluctuations in
the atmosphere, which are known to approximately follow the Kolmogorov
spectrum. The Fourier spectrum is truncated both at some outer scale
(typically known to be between 20 m and 200 m) and some inner scale
(representing the viscous limit, which ends up not affecting the
results).  We then model the atmosphere by a set of these
screens (typically half a dozen). These screens are moved during the
exposure according to a wind velocity vector, and the nature of the
turbulence does not significantly change during an exposure in the
``frozen-screen'' approximation. With these screens, we
start the photons at the top of the atmosphere and then alter their
trajectory according to the derivative of the screen at each
layer. Depending on the time the photon was emitted in the simulation,
the same photon could hit a different part of the screen due to the
wind drift.

After the atmospheric simulation, we continue the photons into the
telescope by reflecting and refracting them when they hit the mirrors
and lenses, using geometric optics techniques. 
%We do this by using well- known geometric optics
%techniques, which is appropriate for large telescopes, such as
%LSST. 
On the surface of the mirrors we put a spectrum of perturbations
that has been obtained by inverting wavefront data from existing
telescopes. We also allow each optic to move according to its six
degrees of freedom within their expected tolerance. The ray-trace uses
extremely fast techniques to find the intercepts on the aspheric
surface and alter the trajectory by reflection or wavelength-dependent 
refraction. We also destroy photons when they pass through
the filter in a Monte Carlo sense according to the wavelength and
angle-dependent transmission function. 
%$The ray-trace for the LSST
%$configuration is shown in \autoref{fig:imsim5}. 
The ray-trace was compared with
commercial ray-trace codes and is accurate to a fraction of a micron. We also add diffraction spikes
due to the telescope spider.

%$\begin{figure}[t]
%$\centerline{\resizebox{!}{4in}{\includegraphics[
%$%viewport=0 0 787 1185,
%$clip]{appendix/imagesim/imsim5_new.jpg}}}
%$\caption{The top panel shows an example of atmospheric turbulence and
%$  the photon ray-tracing scheme.  The middle panel shows a set of
%$  photons being reflected and refracted through mirrors and lensing
%$  using the LSST configuration. The bottom panel shows the photons as
%$  it enters the CCD silicon, the purple lines are the photon
%$  trajectory as it is refracted in the silicon, and the red line shows
%$  the path of the photo-electron after the photon is converted.
%$  Finally, the photons are pixelated to produce an
%$  image. {\bf \XX This figure was taken from a poster.  It should be
%$    redone; remove the top panel, and reduce the verbiage.}\label{fig:imsim5}}
%$\end{figure}

Finally, the photons are ray-traced into the silicon in the
detector. Both the wavelength and temperature dependent conversion
probability and refraction of the silicon is included. The photons are
then converted into photo-electrons that drift to the readout according
to the expected electric field profile. 
%$A set of rays and their
%$interactions in the detector is shown in \autoref{fig:imsim5}. 
The misalignments and surface roughness of the silicon can also be
included. We then pixelate the positions of the photons and can
include blooming, charge saturation, cross-talk, and charge transfer
inefficiency to simulate the readout process. Finally, we build up a
simulated image as the photons reach the readout. We add the read
noise and sky background in a post-processing step.  The sky
background is generated based on a SED for the full moon and a SED for
the dark sky, with an empirically derived angular function for the
Rayleigh scattering of the moon's light.  The background is vignetted
according to the results of ray-trace simulations.

The simulator can generate about 22,000 photons per second on a
typical workstation. For bright stars that saturate, it can simulate
photons much faster since tricks can be used during the simulation to
figure out if a pixel will saturate. Thus, we have a fast simulator
with high fidelity. \autoref{fig:imsim3} shows images of stars with
various components of the simulator turned on or off. \autoref{fig:imsim6} shows a simulated image from one LSST CCD.

\iffalse
[NOT APPROPRIATE FOR THE BOOK]
The code has been massively parallelized. This was particularly
important for the recent massive simulations we have done for Data
Challenge 3. We started with the Purdue CONDOR Pool, which is a large
pool of over 7,000 CPUs that go unused at various points of the day
and use the CONDOR software to submit jobs and/or interrupt jobs on
those unused CPUs.  We chose to submit jobs corresponding to
simulations of a single LSST CCD chip (4096$\times$4096 pixels) as the base
job. An example of a single chip simulations is shown in
\autoref{fig:imsim6}. Below, we list our available simulations.
\fi
\begin{figure}[t]
\centerline{\resizebox{4in}{!}{\includegraphics{appendix/imagesim/psfs.jpg}}}
\caption{Examples of the point-spread-function (PSF) for a single
  star 1 degree off-axis in which various components of the simulator
  are turned on or off. The images show a region $1''$ on a side, and
  the colors distinguish between different regions of the primary that
  the photons hit.  The panels are from top left to bottom right:
  only optical aberrations of the system design, mirror perturbation
  and misalignments, diffusion of charge in the detector, a static
  atmosphere, an atmosphere with wind, and a full atmosphere but a
  perfect telescope. The width of the best-fit Gaussian $\sigma$
  (divide by 30 to get FWHM in arcsec) and the
  ellipticity of each image $e$ are indicated.  Both atmosphere and
  the optics contribute to the ellipticity of the PSF. 
\label{fig:imsim3}}
\end{figure}

\begin{figure}[th!]
\ifthenelse{\boolean{final}}
{\centerline{\resizebox{6in}{!}{\includegraphics{appendix/imagesim/imsim6_gri_binned.jpg}}}
\caption{A simulated image of 15-second exposure of one LSST CCD (4K$\times$4K) with 0.2'' pixels, 0.4'' seeing 
and a field of view $13.7 ' \times 13.7'$, representing
roughly 0.5\% of the LSST focal plane.   
%This CCD is one of 145 fully illuminated 
%CCDs that comprise the LSST focal plane. 
%The image includes all $\sim 3 \times 10^{10}$ photons
%for a 15 second exposure emitted by stars and galaxies in the base
%catalog. 
The brightest stars in 
the image are $\sim 12$ magnitude. An object of brightness $\sim 33$ magnitude would 
make $\sim 1$ photon in a 15 second exposure. 
%The catalog includes objects as faint as  $\sim 43$ magnitude. 
The image is a true color composite of three images, with the $g,  r$,
and $i$  
filters mapped into B, G and R colors respectively. 
Each color channel is on a logarithmic intensity scale.
LSST will produce $\sim2\times10^9$ single-band images of the same size.
\label{fig:imsim6}}}
{\centerline{\resizebox{6in}{!}{\includegraphics{appendix/imagesim/imsim6_small.jpg}}}
\caption{The small simulated image above is one LSST CCD (4K$\times$4K) with 0.2" pixels, 0.4'' seeing 
and a field of view $\sim$13.7 ' $\times \sim13.7$'. This CCD is one of 145 fully illuminated 
CCDs that comprise the LSST focal plane. The image includes all photons ($\sim 3 \times 10^{10}$) 
for a 15 second exposure emitted by stars and galaxies in the base catalog. The brightest stars in 
the image are $\sim$12 magnitude. An object of brightness $\sim$33 magnitude would 
emit $\sim$1 photon in a 15 second exposure. The catalog includes objects as faint as
 $\sim$43 magnitude. The image is a true color composite of three images ({\it g, r} and $i$  
filters mapped into B, G and R colors respectively: display RGB color table). 
Each color channel is on a logarithmic intensity scale.
LSST will produce $\sim2\times10^9$ single-band images of this size.
\label{fig:imsim6}}}
\end{figure}
